# Supplementary material for: Are Large Language Models Geospatially Knowledgeable?
Source: arXiv:2310.13002 source file (2023-10-09)
Supplement: Supplementary file 1 [file main_appendix.tex]

% \clearpage
% \appendix

% \section{Appendix}

% \begin{table}[]
% \centering
% \begin{tabular}{l}
% \hline
% \textbf{Cities}\\
% \hline
% Albany, New York \\
% Albuquerque, New Mexico \\
% Amarillo, Texas	\\
% Atlanta, Georgia	\\
% Austin, Texas	\\
% Baltimore, Maryland	\\
% Bangor, Maine	\\
% Bismarck, North Dakota	\\
% Boise, Idaho	\\
% Boston, Massachusetts	\\
% Buffalo, New York	\\
% Carlsbad, New Mexico	\\
% Charlotte, North Carolina \\
% Cheyenne, Wyoming	\\
% Chicago, Illinois	\\
% Cincinnati, Ohio	\\
% Cleveland, Ohio	\\
% Columbus, Ohio	\\
% Dallas, Texas	\\
% Denver, Colorado	\\
% Des Moines, Iowa	\\
% Detroit, Michigan	\\
% Dubuque, Iowa	\\
% Duluth, Minnesota	\\
% Eastport, Maine	\\
% El Centro, California	\\
% El Paso, Texas	\\
% Eugene, Oregon	\\
% Fargo, North Dakota \\
% Flagstaff, Arizona	\\
% Fort Worth, Texas \\
% Fresno, California \\ \hline
% \end{tabular}
% \begin{tabular}{l}
% \hline
% \textbf{Cities}\\
% \hline
% Grand Junction, Colorado \\
% Grand Rapids, Michigan	\\
% Havre, Montana	\\
% Helena, Montana\\
% Hot Springs, Arkansas	\\
% Houston, Texas	\\
% Idaho Falls, Idaho	\\
% Indianapolis, Indiana	\\
% Jacksonville, Florida	\\
% Juneau, Alaska	\\
% Kansas City, Missouri	\\
% Key West, Florida	\\
% Klamath Falls, Oregon	\\
% Knoxville, Tennessee	\\
% Las Vegas, Nevada	\\
% Lewiston, Idaho	\\
% Long Beach, California	\\
% Los Angeles, California	\\
% Louisville, Kentucky	\\
% Memphis, Tennessee	\\
% Miami, Florida	\\
% Milwaukee, Wisconsin \\
% Minneapolis, Minnesota	 \\
% Montgomery, Alabama	 \\
% Montpelier, Virginia	 \\
% Nashville, Tennessee	 \\
% Newark, New Jersey	\\
% New Haven, Connecticut	 \\
% New Orleans, Louisiana \\
% New York, New York	\\
% Oakland, California	\\
% Oklahoma City, Oklahoma	\\
% Omaha, Nebraska	\\\hline
% \end{tabular}
% \begin{tabular}{l}
% \hline
% \textbf{Cities}\\
% \hline
% Philadelphia, Pennsylvania	\\
% Phoenix, Arizona	\\
% Pierre, South Dakota	\\
% Pittsburgh, Pennsylvania	\\
% Providence, Rhode Island	\\
% Raleigh, North Carolina	\\
% Reno, Nevada	\\
% Richfield, Utah	\\
% Richmond, Virginia	\\
% Roanoke, Virginia	\\
% Sacramento, California	\\
% St. Louis, Missouri	\\
% Salt Lake City, Utah	\\
% San Antonio, Texas	\\
% San Diego, California	\\
% San Francisco, California	\\
% San Jose, California	\\
% Santa Fe, New Mexico	\\
% Savannah, Georgia	\\
% Seattle, Washington State	\\
% Shreveport, Louisiana	\\
% Sioux Falls, South Dakota	\\
% Syracuse, New York	\\
% Tampa, Florida	\\
% Toledo, Ohio	\\
% Tulsa, Oklahoma	\\
% Virginia Beach, Virginia	\\
% Wichita, Kansas	\\
% Wilmington, North Carolina	\\
%  \hspace{1cm} \\ \hline
% \end{tabular}
% \caption{List of cities used in our experiments}
% \label{tab:list_cities}
% \end{table}
